# Supplementary material for: Sampling-Based Motion Planning: A Comparative Review
Source: arXiv:2309.13119 source file (2023-09-22)
Supplement: Supplementary file 1 [file appendix_experimental_method.tex]

\section{Experimental Methodology}
\subsection{Scenario Variation}
\subsubsection{02D Sphere}
Two obstacles, each with radius 1. Initial position in 3D space $x = (1,0,0)$ and $x=(-1,0,0)$. We sample uniformly random position with $\pm 0.2$ in each direction.
